# Supplementary material for: Spider2-V: How Far Are Multimodal Agents From Automating Data Science and Engineering Workflows?
Source: arXiv:2407.10956 source file (2024-07-15)
Supplement: Supplementary file 1 [file datasheet.tex]

\section{Datasheet for \ours}

\subsection{Motivation}

\begin{itemize}
	\item {\bf For what purpose was the dataset created?} Was there a specific
		task in mind? Was there a specific gap that needed to be filled? Please
		provide a description.

The proposal of \ours intends to investigate the capability of existing large language model~(LLM) or vision language model~(VLM) based agents in automating real-world data science and engineering workflows. Task examples in \ours establish two new challenges for LLM/VLM-based data agents: 1) the integration of professional applications, and 2) the incorporation of intensive GUI controls over the web pages of these specialized software.

	\item {\bf Who created the dataset (\textit{e.g.}, which team, research
		group) and on behalf of which entity (\textit{e.g.}, company,
	institution, organization)?}
	
		Ruisheng Cao, Fangyu Lei, Haoyuan Wu, Jixuan Chen, Yeqiao Fu, Hongcheng Gao, Xinzhuang Xiong, Hanchong Zhang, Yuchen Mao, Wenjing Hu, Tianbao Xie, Hongshen Xu, Danyang Zhang, Lu Chen, Kai Yu and Tao Yu, on behalf of
		1) XLang Lab of the University of Hong Kong and 2) X-LANCE Lab of SJTU AI Institute, create the environment and the task set.

	%\item {\bf Who funded the creation of the dataset?} If there is an
		%associated grant, please provide the name of the grantor and the grant
		%name and number.
%
		%TODO % TODO

	%\item {\bf Any other comments?}
\end{itemize}

\subsection{Composition}

\begin{itemize}
	\item {\bf What do the instances that comprise the dataset represent
		(\textit{e.g.}, documents, photos, people, countries)?} Are there
		multiple types of instances (\textit{e.g.}, movies, users, and ratings;
		people and interactions between them; nodes and edges)? Please provide
		a description.

    Each instance in \ours represents a real-world data science and engineering task which can be fulfilled by data scientists on a computer. These tasks cover the entire data pipeline, including 1) data warehousing, 2) data transformation, 3) data ingestion and integration, 4) data analysis and visualization, 5) traditional data processing, 6) data orchestration, and 7) IT service management.

	\item {\bf How many instances are there in total (of each type, if
		appropriate)?}

		We totally instantiate \tasknum tasks spanning across $20$ professional applications and the entire data pipeline. We also provide a document warehouse containing \docnum documents which are crawled and pre-processed from the official websites of these professional data science and engineering software to support retrieval augmented agent framework.

	\item {\bf Does the dataset contain all possible instances or is it a
		sample (not necessarily random) of instances from a larger set?} If the
		dataset is a sample, then what is the larger set? Is the sample
		representative of the larger set (\textit{e.g.}, geographic coverage)?
		If so, please describe how this representativeness was validated\slash
		verified. If it is not representative of the larger set, please
		describe why not (\textit{e.g.}, to cover a more diverse range of
		instances, because instances were withheld or unavailable).

		The entire task set contains \tasknum examples which stem from the following $3$ sources: 1) dataset SheetCopilot~\citep{sheetcopilot} from which we randomly sample $31$ tasks, 2) benchmark WorkArena~\citep{workarena} from which we sample one for each distinct task type, and 3) official tutorials or guides on professional applications~(e.g., {\tt dbt}, {\tt Airflow}, {\tt Dagster}, {\tt Superset}, etc.). During construction, we focus on the task diversity and reality. And each task sample goes through strict manual cross-validation by at least two annotators~(see \cref{sec:annotation}).

	\item {\bf What data does each instance consist of?} ``Raw'' data
		(\textit{e.g.}, unprocessed text or images) or features? In either case,
		please provide a description.

		Each instance in \ours includes a text-format natural language instruction~(task goal), two lists of functions defining how to set up the initial environment and how to evaluate the final outcome respectively, as well as some other task metadata. All information is organized in the JSON format. They can be directly loaded by the provided environment and support interactive and continuous communication with data agents until task completion. All types of auxiliary media~({\it e.g.}, files, images, archives or scripts associated with different tasks) are provided in company with the raw JSON data.

	\item {\bf Is there a label or target associated with each instance?} If so,
		please provide a description.

  Yes. For each instance, it includes a task goal, methods of how to recover the initial environment and how to evaluate whether the task is completed successfully.

	\item {\bf Is any information missing from individual instances?} If so,
		please provide a description, explaining why this information is
		missing (\textit{e.g.}, because it was unavailable). This does not
		include intentionally removed information, but might include,
		\textit{e.g.}, redacted text.

		For part of the task instances, we require the user to provide a personal account of specific professional applications~({\it e.g.}, {\tt BigQuery} and {\tt Snowflake}). We can not provide a public account. The reason is that, if multiple users share one trial account, the situation may occur that when one person just finished the task using his/her data agent and prepare to evaluate the results, another person happens to reset the environment for the same task, thus destroying all finished states in the cloud workspace of this real account. However, we do provide templates and instructions about how to register and use these real accounts for \ours.

	\item {\bf Are there any errors, sources of noise, or redundancies in the
		dataset?} If so, please provide a description.

		Currently, no. Errors and noise are eliminated via strict cross-validation by at least two annotators. Versions of different software or libraries are fixed for robustness and consistency. Redundancies should not exist since each task sample is uniquely selected for diversity.

	\item {\bf Is the dataset self-contained, or does it link to or otherwise
rely on external resources (\textit{e.g.}, websites, tweets, other datasets)?}
If it links to or relies on external resources, a) are there guarantees that
they will exist, and remain constant, over time; b) are there official archival
versions of the complete dataset (\textit{i.e.}, including the external
resources as they existed at the time the dataset was created); c) are there
any restrictions (\textit{e.g.}, licenses, fees) associated with any of the
external resources that might apply to a dataset consumer? Please provide
descriptions of all external resources and any restrictions associated with
them, as well as links or other access points, as appropriate.

	\ours includes a subset of two existing benchmarks, namely SheetCopilot~\cite{sheetcopilot} and WorkArena~\citep{workarena}. In response to sub-questions: a) Data has been downloaded locally and transformed to the target format of \ours. b) Yes. \ours archives all the annotations. c) These two benchmarks are released under GPL-3.0 license and Apache-2.0 license respectively. Therefore, we have access to them and do not violate any protocol.

	\item {\bf Does the dataset contain data that might be considered
		confidential (\textit{e.g.}, data that is protected by legal privilege
	or by doctor–patient confidentiality, data that includes the content of
	individuals' non-public communications)?} If so, please provide a
	description.

		No.

	\item {\bf Does the dataset contain data that, if viewed directly, might be
		offensive, insulting, threatening, or might otherwise cause anxiety?}
		If so, please describe why.

		No.

	\item {\bf Does the dataset identify any subpopulations (\textit{e.g.}, by
		age, gender)?} If so, please describe how these subpopulations are
		identified and provide a description of their respective distributions
		within the dataset.

		No.

	\item {\bf Is it possible to identify individuals (\textit{i.e.}, one or
		more natural persons), either directly or indirectly (\textit{i.e.}, in
	combination with other data) from the dataset?} If so, please describe how.

		No. Only the research group of \ours may be identified, because we use the benchmark name in some task instances~({\it e.g.}, file name or folder called ``{\tt Spider2}'') for demonstration use case. For other individuals, it is impossible.

	\item {\bf Does the dataset contain data that might be considered sensitive
			in any way (\textit{e.g.}, data that reveals race or ethnic
				origins, sexual orientations, religious beliefs, political
				opinions or union memberships, or locations; financial or
				health data; biometric or genetic data; forms of government
		identification, such as social security numbers; criminal history)?} If
		so, please provide a description.

		No.
	%\item {\bf Any other comments?}
\end{itemize}

\subsection{Collection Process}

\begin{itemize}
	\item {\bf How was the data associated with each instance acquired?} Was
		the data directly observable (\textit{e.g.}, raw text, movie ratings),
		reported by subjects (\textit{e.g.}, survey responses), or indirectly
		inferred\slash derived from other data (\textit{e.g.}, part-of-speech
		tags, model-based guesses for age or language)?  If the data was
		reported by subjects or indirectly inferred\slash derived from other
		data, was the data validated\slash verified? If so, please describe
		how.

		All data and information used in \ours are directly observable from 1) existing benchmarks~(SheetCopilot and WorkArena) and 2) websites of official tutorials for various professional applications. Indeed, the JSON-format metadata of each task contains one field ``{source}'' indicating where the data comes from.

	\item {\bf What mechanisms or procedures were used to collect the data
		(\textit{e.g.}, hardware apparatuses or sensors, manual human curation,
	software programs, software APIs)?} How were these mechanisms or procedures
	validated?
	
		\ours is developed with a virtual machine based computer desktop. And tasks are annotated through manual human curation and manual cross validation on the virtual machine. The detailed procedure~(including the verification step) is summarized and demonstrated with one concrete example in \cref{sec:annotation}.

	\item {\bf If the dataset is a sample from a larger set, what was the
		sampling strategy (\textit{e.g.}, deterministic, probabilistic with
	specific sampling probabilities)?}

        For the subset that stems from existing benchmarks, we adopt uniform sampling for different task types to ensure diversity. For the main part which originates from official tutorials of various professional applications, we adopt breadth-first-search to collect diverse topics~(removing duplicates). Then, we iterate through these tutorials and filter those tutorials that can not be instantiated.

	\item {\bf Who was involved in the data collection process (\textit{e.g.},
		students, crowdworkers, contractors) and how were they compensated
	(\textit{e.g.}, how much were crowdworkers paid)?}

		All the development of the environment and task
		set are completed by the authors.

	\item {\bf Over what timeframe was the data collected?} Does this timeframe
		match the creation timeframe of the data associated with the instances
		(\textit{e.g.}, recent crawl of old news articles)? If not, please
		describe the timeframe in which the data associated with the instances
		was created.

		The task set is collected from official tutorials of professional applications in Table~\ref{fig:task_categories}
		from Jan.\ 20th, 2024 to Jun.\ 2nd, 2024.

	%\item {\bf Were any ethical review processes conducted (e.g., by an
		%institutional review board)?} If so, please provide a description of
		%these review processes, including the outcomes, as well as a link or
		%other access point to any supporting documentation.

	\item {\bf Did you collect the data from the individuals in question
		directly, or obtain it via third parties or other sources (e.g.,
	websites)?}

		Data is collected from official websites of various professional applications. For the complete checklist of all websites, see Table~\ref{tab:docs}.

	\item {\bf Were the individuals in question notified about the data
		collection?} If so, please describe (or show with screenshots or other
		information) how notice was provided, and provide a link or other
		access point to, or otherwise reproduce, the exact language of the
		notification itself.

		Not applicable. We do not collect data from individuals.

	\item {\bf Did the individuals in question consent to the collection and
		use of their data?} If so, please describe (or show with screenshots or
		other information) how consent was requested and provided, and provide
		a link or other access point to, or otherwise reproduce, the exact
		language to which the individuals consented.

		Not applicable. We do not collect data from individuals.
  
	\item {\bf If consent was obtained, were the consenting individuals
		provided with a mechanism to revoke their consent in the future or for
	certain uses?} If so, please provide a description, as well as a link or
	other access point to the mechanism (if appropriate).

	Not applicable. We do not collect data from individuals.
  
	%\item {\bf Has an analysis of the potential impact of the dataset and its
		%use on data subjects (\textit{e.g.}, a data protection impact analysis)
	%been conducted?} If so, please provide a description of this analysis,
	%including the outcomes, as well as a link or other access point to any
	%supporting documentation.
	%\item {\bf Any other comments?}
\end{itemize}

\subsection{Uses}

\begin{itemize}
	\item {\bf Has the dataset been used for any tasks already?} If so, please
		provide a description.

		Data agents based on different LLMs and VLMs have been evaluated on \ours in this paper.

	\item {\bf Is there a repository that links to any or all papers or systems
		that use the dataset?} If so, please provide a link or other access
		point.
		
		Yes. We construct a project website~(\url{https://spider2-v.github.io/}) tracking results for \ours.

	%\item {\bf What (other) tasks could the dataset be used for?}
	\item {\bf Is there anything about the composition of the dataset or the
		way it was collected and preprocessed\slash cleaned\slash labeled that
	might impact future uses?} For example, is there anything that a dataset
	consumer might need to know to avoid uses that could result in unfair
	treatment of individuals or groups (\textit{e.g.}, stereotyping, quality of
	service issues) or other risks or harms (\textit{e.g.}, legal risks,
	financial harms)? If so, please provide a description. Is there anything a
	dataset consumer could do to mitigate these risks or harms?

		No.

	%\item {\bf Are there tasks for which the dataset should not be used?} If so,
		%please provide a description.
	%\item {\bf Any other comments?}
\end{itemize}

\subsection{Distribution}

\begin{itemize}
	\item {\bf Will the dataset be distributed to third parties outside of the
		entity (\textit{e.g.}, company, institution, organization) on behalf of
	which the dataset was created?} If so, please provide a description.

		Yes. Both the environment, the task set and experiment code will be open-sourced in Github \url{https://github.com/xlang-ai/Spider2-V}.

	\item {\bf How will the dataset will be distributed (\textit{e.g.}, tarball
		on website, API, GitHub)?} Does the dataset have a digital object
		identifier (DOI)?

		The platform is open-sourced in GitHub~\url{https://github.com/xlang-ai/Spider2-V}. The task set is also released at
		Hugging Face. We do not apply for a DOI.

	\item {\bf When will the dataset be distributed?}

		Both the executable environment and the task set have already been made public.

	\item {\bf Will the dataset be distributed under a copyright or other
		intellectual property (IP) license, and\slash or under applicable terms
	of use (ToU)?} If so, please describe this license and\slash or ToU, and
	provide a link or other access point to, or otherwise reproduce, any
	relevant licensing terms or ToU, as well as any fees associated with these
	restrictions.

		\ours is open-sourced under
		Apached-2.0 license.

	\item {\bf Have any third parties imposed IP-based or other restrictions on
		the data associated with the instances?} If so, please describe these
		restrictions, and provide a link or other access point to, or otherwise
		reproduce, any relevant licensing terms, as well as any fees associated
		with these restrictions.

		Yes. IPs in some countries do not have access to the service delivered by some professional applications~({\it e.g.}, {\tt BigQuery} and {\tt Snowflake}) involved in \ours. However, we do provide the solution to resolve this issue by setting the network proxy. And this constrained task subset is marked as a separate split only for interested users.

	\item {\bf Do any export controls or other regulatory restrictions apply to
		the dataset or to individual instances?} If so, please describe these
		restrictions, and provide a link or other access point to, or otherwise
		reproduce, any supporting documentation.

		No.

	%\item {\bf Any other comments?}
\end{itemize}

\subsection{Maintenance}

\begin{itemize}
	\item {\bf Who will be supporting\slash hosting\slash maintaining the
		dataset?}

		The authors will support, host, and maintain both the environment and the task set of \ours.

	\item {\bf How can the owner\slash curator\slash manager of the dataset be
		contacted (\textit{e.g.}, email address)?}

		Issues and discussions on GitHub and Hugging Face are welcome. One can
		also seek help from Ruisheng Cao ({\tt ruishengcao@gmail.com}), and Tao Yu ({\tt
		tao.yu.nlp@gmail.com}).

	\item {\bf Is there an erratum?} If so, please provide a link or other
		access point.

		Currently, no. Errata will be anounced if there is any in future.

	\item {\bf Will the dataset be updated (\textit{e.g.}, to correct labeling
		errors, add new instances, delete instances)?} If so, please describe
		how often, by whom, and how updates will be communicated to dataset
		consumers (\textit{e.g.}, mailing list, GitHub)?

		\ours will be continuously developed and maintained.
		Updates will be released on GitHub and project website from time to time. Errata may be
		released to correct errors if there is any in future.

	\item {\bf If the dataset relates to people, are there applicable limits on
		the retention of the data associated with the instances (\textit{e.g.},
	were the individuals in question told that their data would be retained for
	a fixed period of time and then deleted)?} If so, please describe these
	limits and explain how they will be enforced.

		No.

	\item {\bf Will older versions of the dataset continue to be
		supported\slash hosted\slash maintained?} If so, please describe how.
		If not, please describe how its obsolescence will be communicated to
		dataset consumers.

		Yes. Old versions of \ours can be accessed through
		GitHub and Hugging Face, respectively.

	\item {\bf If others want to extend\slash augment\slash build on\slash
		contribute to the dataset, is there a mechanism for them to do so?} If
		so, please provide a description. Will these contributions be
		validated/verified? If so, please describe how. If not, why not? Is
		there a process for communicating\slash distributing these
		contributions to dataset consumers? If so, please provide a
		description.

		We sincerely welcome that one can contribute features or report bugs
		for \ours through the mechanisms like pull request, issues,
		\textit{etc}.\ on GitHub. If new environments or task sets are crafted,
		it will be welcome that the creators notify the authors through e-mail
		or GitHub, so that we can update the indices of available task sets.
		
	%\item {\bf Any other comments?}
\end{itemize}
