# Supplementary material for: Spider2-V: How Far Are Multimodal Agents From Automating Data Science and Engineering Workflows?
Source: arXiv:2407.10956 source file (2024-07-15)
Supplement: Supplementary file 2 [file settings.tex]

\section{Details of Experiment Settings}
We utilize the version {\tt gpt-4o-2024-05-13} for GPT-4o and {\tt gpt-4-1106-vision-preview} for GPT-4V respectively. Note that, results could be updated from time since they are close-sourced. For all experiments except the ablation study, we set the temperature to $0.5$ and top\_p to $0.9$, the maximum length of {\tt a11ytree} in each turn to $5000$ tokens, and the maximum output tokens to $1500$. Besides, the maximum interaction turns is fixed to $15$ and the maximum running time is limited to one hour for all tasks since the agent could get stuck in some unexpected cases. Due to context length restriction, we also set the maximum number of history window to $3$ interaction turns.
